# Supplementary material for: Coverage-aware Semantic Representation Learning for Underrepresented Visual Concepts
Source: arXiv:2602.16917 source file (2026-09-27)
Supplement: Supplementary file 1 [file supp-milk10k-clinical-classification.tex]

\begin{table*}[!t]
    \centering
    \caption{Performance on the MILK10k (Clinic) dataset.}
    \label{tab:supp-benchmark-milk10k-clinic}
   \resizebox{\linewidth}{!}
    {
        \begin{tabular}{lllllll}
        \toprule
            Model & Accuracy & Precision &	Recall & F1 & AUC & Per-Class Acc \\
        \midrule
            % Baseline (ENet-B0) & 0.9218 & 0.5351 & 0.6778 & 0.5980 & 0.9267 \\
            ENet-B0 & 0.9208 &  0.5778 &  0.2889 &  0.3852 &  0.9151 & [0.98016701 0.28888889]  \\
            ViT & 0.9198 &  0.6500 &  0.1444 &  0.2364 &  0.8839 & [0.99269311 0.14444444]  \\
          %   + Class balanced loss \\
          %   + Focal loss \\
          %   + Asymmetric loss \\
          %   + DAR & 0.9208 & 0.5310 & 0.6667 & 0.5911 & 0.9328 \\
          %   + DAR+DRB & 0.9389 & 0.6512 & 0.6222 & 0.6364 & 0.9327 \\
          \midrule
            SemCovNet (ours) &  \\
            + $\mathcal{L}_{dva}$ & 0.9399 & 0.7288 & 0.4778 & 0.5772 & 0.9013 & [0.97494781 0.42222222] \\
            + $\mathcal{L}_{total}$ & \\
        \bottomrule
        \end{tabular}
    }
\end{table*}
