# Supplementary material for: Coverage-aware Semantic Representation Learning for Underrepresented Visual Concepts
Source: arXiv:2602.16917 source file (2026-09-27)
Supplement: Supplementary file 2 [file supp-milk10k-derm-classification.tex]

\begin{table*}[!t]
    \centering
    \caption{Performance on the MILK10k (Dermoscopic) dataset.}
    \label{tab:supp-benchmark-milk10k-derm}
   \resizebox{\linewidth}{!}
    {
        \begin{tabular}{lllllll}
        \toprule
            Model & Accuracy & Precision &	Recall & F1 & AUC & Per-Class Acc \\
        \midrule
            % Baseline (ENet-B0) & 0.9218 & 0.5351 & 0.6778 & 0.5980 & 0.9267 \\
            ENet-B0 & 0.9208 & 0.5385 & 0.5444 & 0.5414 & 0.9114 & [0.95615866 0.54444444]  \\
            ViT & 0.9122 & 0.4857 & 0.3778 & 0.4250 & 0.9032 &  [0.96242171 0.37777778] \\
          %   + Class balanced loss \\
          %   + Focal loss \\
          %   + Asymmetric loss \\
          %   + DAR & 0.9208 & 0.5310 & 0.6667 & 0.5911 & 0.9328 \\
          %   + DAR+DRB & 0.9389 & 0.6512 & 0.6222 & 0.6364 & 0.9327 \\
          % \midrule
          %   + SDM+DAM(Early) & 0.9170 & 0.5113 & 0.7556 & 0.6099 & 0.9235 \\
          %   + SDM+DAM(Mid) & 0.9284 & 0.5758 & 0.6333 & 0.6032 & 0.9111 \\
          %   + $\mathcal{L}_{desc}$\\
        \midrule
            SemCovNet (ours) &  \\
            + $\mathcal{L}_{dva}$ & \\
            + $\mathcal{L}_{total}$ & \\
        \bottomrule
        \end{tabular}
    }
\end{table*}
